# Supplementary material for: Phase transitions of hybrid perovskites simulated by machine-learning force fields trained on-the-fly with Bayesian inference
Source: arXiv:1903.09613 ancillary file (2019-03-22)
Supplement: Supplementary file 1 [file Supplementary-Materials_Jinnouchi_2019.pdf]

**Supplementary Materials for**

# Phase transitions of hybrid perovskites simulated by machine-learning force fields trained on-the-fly with Bayesian inference

Ryosuke Jinnouchi,[1,2] Jonathan Lahnsteiner,[1] Ferenc Karsai,[3]
Georg Kresse[1,3] and Menno Bokdam[1]

1. University of Vienna, Faculty of Physicf and Center for Computational Materials Sciences, Sensengasse 8/12, 1090 Wien, Austria.
2. Toyota Central R&D Labs., Inc., 41-1 Yokomichi, Nagakute, Aichi 480-1192, Japan.
3. VASP Software GmbH, Sensengasse 8, Vienna, Austria.

**Contents**

**A. On-the-fly machine-learning force-field generation**
**B. Models and parameters for training**
**C. Efficiency and accuracy**
**D. Simulations of phase transitions using force fields**
**E. Order parameters**
**F. Reorientation time of MA molecules**
**G. Ionic radii and Goldschmidt tolerance factors**
**H. Supplementary Movies**

## A. On-the-fly machine learning force-field generation

In our scheme, a MLFF is generated on the fly during the FP MD simulations, as outlined below:

1) Energy, forces and the stress tensor of a newly appearing structure and their errors are predicted on the basis of Bayesian interference using the yet available force field.
2) If the predicted errors are larger than a chosen threshold, FP calculations are performed to obtain data on the new sample structure. Otherwise, the algorithm continues with step 4).
3) If the number of new sample structures reaches five, the sampled data is sparsified, and the force field is refined. This blocking increases the computational efficiency.
4) The equations of motions are integrated by using the forces and the stress tensor provided by the MLFF or the FP calculation. Return to step 1).

This scheme consists of several key methodologies and parameters: accurate description of the potential energy surface, optimization of parameters, error estimations, and a proper setting of the threshold for the estimated errors to decide whether to perform the FP calculations or not. For each part, new methods and numerical techniques have been developed in order to make the algorithm efficient, systematic and robust. The core features and the used parameters are explained in the following subsections.

*Potential energy surface and descriptor*

For the description of the potential energy surface, we adopt a method similar to the Gaussian approximation potential (GAP) (Ref.[2] in the main text) with the SOAP (Ref.[22] in the main text) as a similarity measure. However, some new features are present in our scheme. In order to explain these features in a clear manner, we reformulate the potential energy surface and its descriptor.

In GAP, the potential energy surface $U$ of a system with $N_\mathrm{a}$ atoms is decomposed into atomic energies $U_i$ as follows,

$$U = \sum_{i=1}^{N_\mathrm{a}} U_i. \tag{A1}$$

$U_i$ is assumed to be fully determined by the local chemical environment surrounding the $i$th atom. As a representation of the local chemical environment, an atomic distribution would be reasonable. In SOAP, this distribution is defined as a probability $\rho_i$ to find a single atom at position $\mathbf{r}$ within a certain cutoff radius $R_\mathrm{cut}$ from the $i$th atom, and it is obtained as follows,

$$\rho_i(\mathbf{r}) = \sum_{j=1}^{N_\mathrm{a}} f_\mathrm{cut}(r_{ji})\, g(\mathbf{r} - \mathbf{r}_j + \mathbf{r}_i), \tag{A2}$$

where $f_\mathrm{cut}$ is a cutoff function that is introduced to smoothly cancel out contributions outside the radius $R_\mathrm{cut}$, $\mathbf{r}_i$ is the position of the $i$th atom, $r_{ji}=|\mathbf{r}_i-\mathbf{r}_j|$ is the distance between two atoms, and $g$ is the smoothed distribution, which is described as a Gaussian function as follows,

$$g(\mathbf{r}) = \frac{1}{\left(\sqrt{2\sigma_{\text{atom}}^2\pi}\right)^3}\exp\left(-\frac{|\mathbf{r}|^2}{2\sigma_{\text{atom}}^2}\right). \quad \text{(A3)}$$

In our implementation, the cosine function proposed by Behler and Parrinello (see Ref.[1] in the main text) is used as the cutoff function. As already discussed in literature (see Ref.[22] in the main text), the function $\rho_i$ does not satisfy the rotational invariance, and therefore, it is not advisable to directly use it as the descriptor of $U_i$ which must satisfy the rotational invariance. For this reason, rotationally invariant descriptors need to be constructed from $\rho_i$.

In the developed algorithm, we propose to combine two descriptors as the representation of the local chemical environment. One is the simplest possible rotationally invariant descriptor, that is a pairwise radial distribution written as follows,

$$\rho_i^{(2)}(r) = \frac{1}{4\pi}\int \rho_i(r\hat{\mathbf{r}})d\hat{\mathbf{r}}. \quad \text{(A4)}$$

The other is a probability to find an atom $j$ at a distance $r$ from the $i$th atom and another atom $k$ at a distance $s$ from the $i$th atom along a direction specified by an angle $\angle kij = \theta$. This probability, which we call angular distribution in this study, is described as follows,

$$\rho_i^{(3)}(r,s,\theta) = \iint \delta(\hat{\mathbf{r}}\cdot\hat{\mathbf{s}} - \cos\theta)\,\rho_i(r\hat{\mathbf{r}})\rho_i^*(s\hat{\mathbf{s}})d\hat{\mathbf{r}}d\hat{\mathbf{s}}. \quad \text{(A5)}$$

This second descriptor is equivalent to the power spectrum used in practical applications of SOAP [1–4]. The equivalence can be shown by converting Eq. (A5) using the expansion coefficients $c^i_{nlm}$ defined as follows,

$$\rho_i(\mathbf{r}) = \sum_{n=1}^{N_\text{R}}\sum_{l=0}^{L_\text{max}}\sum_{m=-l}^{l} c^i_{nlm}\chi_{nl}(r)\,Y_{lm}(\hat{\mathbf{r}}), \quad \text{(A6)}$$

where $\chi_{nl}$ denotes the orthonormal radial basis set, which consists of spherical Bessel functions in our implementation, and $Y_{lm}$ denotes the spherical harmonics. The converted equations for Eqs. (A4) and (A5) are summarized as follows,

$$\rho_i^{(2)}(r) = \frac{1}{\sqrt{4\pi}}\sum_{n=1}^{N_\text{R}} c^i_n\chi_{n0}(r), \quad \text{(A7)}$$

$$c^i_n = c^i_{n00}, \quad \text{(A8)}$$

$$\rho_i^{(3)}(r,s,\theta) = \sum_{n=1}^{N_\text{R}}\sum_{\nu=1}^{N_\text{R}}\sum_{l=0}^{L_\text{max}}\sqrt{\frac{2l+1}{2}}\,p^i_{n\nu l}\chi_{nl}(r)\chi_{\nu l}(s)P_l(\cos\theta), \quad \text{(A9)}$$

$$p^i_{n\nu l} = \sqrt{\frac{8\pi^2}{2l+1}}\sum_{m=-l}^{l} c^i_{nlm}c^{i*}_{\nu lm}, \quad \text{(A10)}$$

where $P_l$ are Legendre polynomials. Eq. (A10) is the same as the conventional equation for the power spectrum of SOAP (see Ref.[22] in the main text), and Eq. (A9) indicates that the power spectrum $p^i_{n\nu l}$ corresponds to the expansion coefficients of the angular distribution $\rho_i^{(3)}$ with respect to the orthonormal basis sets. Thus, the power spectrum contains the same information as the angular distribution.

The angular distribution contains radial information too, but its computation requires significantly more computational time than the radial distribution, particularly when a large cutoff radius is used to include long-range interactions. On the other hand, physical and chemical intuition

**Table A1** Parameters of radial and angular descriptors.

| Parameter | Value or type | Parameter | Value or type |
|---|---|---|---|
| $\sigma_{atom}$ | 0.5 Å | $\chi_{nl}$ | spherical Bessel function |
| $R_{cut}$ (radial) | 6 Å | $N_R$ (radial) | 6 |
| $R_{cut}$ (angular) | 4 Å for $MAPbI_3$<br>5 Å for others | $N_R$ (angular) | 7 for $MAPbI_3$<br>9 for others |
| $\alpha^{(2)}$ | 0.5 | $L_{max}$ | 6 |
| $\alpha^{(3)}$ | 0.5 | $\zeta^{(3)}$ | 4 |

indicates that long-range interactions can be reasonably approximated by radial functions, such as Coulomb and Lennard-Jones functions. Taking into account these facts, we propose to combine the radial distribution with a large cutoff radius and the angular distribution with a short cutoff radius.

The radial and angular distributions are used as the descriptors of $U_i$. This means that $U_i$ is described as a functional of $\rho_i^{(2)}$ and $\rho_i^{(3)}$,

$$U_i = F\left[\rho_i^{(2)}, \rho_i^{(3)}\right]. \tag{A11}$$

One can exactly express this functional by superposing delta-functions in the multi-dimensional space spanned by the descriptor vector $\mathbf{X}$ as follows,

$$F\left[\rho_i^{(2)}, \rho_i^{(3)}\right] = \sum_{i_B=1}^{N_B} w_{i_B} \delta\left(\mathbf{X}_i - \mathbf{X}_{i_B}\right), \tag{A12}$$

where the descriptor vector $\mathbf{X}_i$ contains $c^i_n$ and $p^i_{n\nu l}$ as its elements, and $w_{i_B}$ is regarded as the atomic energy at the local reference configuration $\mathbf{X}_{i_B}$. In practice, in order to efficiently interpolate the limited number of the local reference configurations, the delta function needs to be broadened by using a Gaussian or polynomial function. In this study, the following polynomial function is used

$$F\left[\rho_i^{(2)}, \rho_i^{(3)}\right] = \sum_{i_B=1}^{N_B} w_{i_B} K\left(\mathbf{X}_i, \mathbf{X}_{i_B}\right), \tag{A13}$$

$$K\left(\mathbf{X}_i, \mathbf{X}_{i_B}\right) = \left[\alpha^{(2)}\left(\mathbf{X}_i^{(2)} \cdot \mathbf{X}_{i_B}^{(2)}\right) + \alpha^{(3)}\left(\overline{\mathbf{X}}_i^{(3)} \cdot \overline{\mathbf{X}}_{i_B}^{(3)}\right)^{\zeta^{(3)}}\right]. \tag{A14}$$

Here, $\mathbf{X}_i^{(2)}$ and $\mathbf{X}_i^{(3)}$ are the vectors containing $c^i_n$ and $p^i_{n\nu l}$, respectively, as their elements, $\overline{\mathbf{X}}_i^{(3)}$ denotes a normalized vector of $\mathbf{X}_i^{(3)}$, $\alpha^{(2)}$ and $\alpha^{(3)}$ are the weighting parameters, and $\zeta^{(3)}$ is the parameter to control the sharpness of $K$. The second term in Eq. (A14) is identical to the SOAP. The first term describes pairwise linear radial interactions, which are suited to describe the long-range interactions. In Table A1, the used parameters are tabulated.

*Predictions of energy, force and stress tensor and their uncertainty*

In the following we distinguish between a *structure dataset* and a *local configuration*. The structure dataset consists of the Bravais lattice, the atomic positions, the total energy, forces and stress tensor for a specific structure calculated by FP. For each atom in the structure, a local

configuration around this atom can be calculated. This local configuration can be mapped onto a set of descriptors describing the local environment of each atom.

Equations (A1), (A11) and (A13) indicate that the potential energy, forces and stress tensor on a given structure are described as linear functions of the parameters $w_{i_\mathrm{B}}$ as follows,

$$\mathbf{y} = \boldsymbol{\phi}\mathbf{w}. \tag{A15}$$

Here, the vector $\mathbf{y}$ denotes an $m$=1+3$N_\mathrm{a}$+6 dimensional vector composed of the dimensionless energy, forces and stress tensor, which are obtained by dividing their original values by the standard deviations of FP energies, forces and stress tensors in reference structure datasets. The vector $\mathbf{w}$ denotes an $N_\mathrm{B}$ dimensional vector composed of the coefficient $w_{i_\mathrm{B}}$, and $\boldsymbol{\phi}$ is an $m$×$N_\mathrm{B}$ matrix derived from Eqs. (A1), (A11) and (A13). For calculating $\mathbf{y}$, one needs to select the reference structures that provide the local reference configurations $\mathbf{X}_{i_\mathrm{B}}$. The regression coefficients $\mathbf{w}$ also need to be determined. The reference structures are selected on the fly during MD simulations as will be explained later on. After the selection, the regression coefficients $\mathbf{w}$ are also optimized on the fly to reproduce the FP energies, forces and stress tensors of the selected structures. In our scheme, this optimization is carried out by a Bayesian linear-regression method (see Ref. [24] in the main text). In this method, a probability to find $\mathbf{w}$ after observing the FP energies, forces and stress tensors in the reference structure datasets is described as a Gaussian distribution centered at $\bar{\mathbf{w}}$ with a covariance matrix of $\boldsymbol{\Sigma}$ on the basis of the Bayesian theorem. Equations for $\bar{\mathbf{w}}$ and $\boldsymbol{\Sigma}$ are written as follows,

$$\bar{\mathbf{w}} = \frac{1}{\sigma_\mathrm{v}^2}\boldsymbol{\Sigma}\boldsymbol{\Phi}^\mathrm{T}\mathbf{T}, \tag{A16}$$

$$\boldsymbol{\Sigma}^{-1} = \frac{1}{\sigma_\mathrm{w}^2}\mathbf{I} + \frac{1}{\sigma_\mathrm{v}^2}\boldsymbol{\Phi}^\mathrm{T}\boldsymbol{\Phi}. \tag{A17}$$

Here, $\mathbf{T}$ denotes an $M$=$mN_\mathrm{D}$ dimensional vector collecting all FP energies, forces and stress tensors in the $N_\mathrm{D}$ reference structures (made dimensionless by division by the standard deviations). $\boldsymbol{\Phi}$ is an $M$×$N_\mathrm{B}$ design matrix comprised of all matrices $\boldsymbol{\phi}$ for the selected reference structures. $\mathbf{I}$ denotes the unit matrix. By this posterior distribution of $\mathbf{w}$, the dimensionless energy, forces and stress tensor on a new structure are also described as a Gaussian distribution centered at $\bar{\mathbf{y}}$ with a covariance matrix $\boldsymbol{\sigma}$ written as follows,

$$\bar{\mathbf{y}} = \boldsymbol{\phi}\bar{\mathbf{w}}, \tag{A18}$$

$$\boldsymbol{\sigma} = \sigma_\mathrm{v}^2\mathbf{I} + \boldsymbol{\phi}^\mathrm{T}\boldsymbol{\Sigma}\boldsymbol{\phi}. \tag{A19}$$

The mean vector $\bar{\mathbf{y}}$ contains the predicted energy, forces and stress tensor. The equation (A19) is the same as Eq. (2) in the main text, and the diagonal elements in the matrix $\boldsymbol{\sigma}$ correspond to the uncertainty in the prediction. The ratio of $\sigma_\mathrm{v}^2$ to $\sigma_\mathrm{w}^2$ is equivalent to the Tikhonov regularization parameter in the ridge regression, and its optimization is important to balance the accuracy and robustness of the developing force field. In our scheme, the parameters are optimized by the evidence approximation (see also Ref.[24] in the main text).

In addition to the Bayesian error estimation defined as (A19), we use the spilling factor [5] for the error estimation

$$s_i = 1 - \frac{\sum_{i_{\mathrm{B}}=1}^{N_{\mathrm{B}}} \sum_{i'_{\mathrm{B}}=1}^{N_{\mathrm{B}}} K\left(\mathbf{x}_i, \mathbf{x}_{i_{\mathrm{B}}}\right) K^{-1}\left(\mathbf{x}_{i_{\mathrm{B}}}, \mathbf{x}_{i'_{\mathrm{B}}}\right) K\left(\mathbf{x}_{i'_{\mathrm{B}}}, \mathbf{x}_i\right)}{K(\mathbf{x}_i, \mathbf{x}_i)}. \quad \text{(A20)}$$

Here, the equation is slightly modified from its original equation in order to make it suitable to the non-normalized matrix $K$ like Eq. (A14).

Each error estimator has its advantages and disadvantages. By combining these two estimators, the error estimation process becomes reliable and applicable to a wide variety of materials.

*Decision whether to perform the FP calculation or not*

One of the most significant processes in our on-the-fly scheme is the decision whether to perform FP calculations or not. This process significantly affects the quality of the reference structure datasets as well as the efficiency of the computations. The decision is done on the basis of the estimated errors provided by Eqs. (A19) and (A20) and the history of the previous sampling. First, the machine checks the previous sampling step. If the MD step is within 10 steps from the previous sampling step, the machine simply bypasses the FP calculation. This process avoids too dense samplings within a narrow phase space. If 10 MD steps passed since the previous sampling step, the machine examines the Bayesian errors for the forces and the spilling factors. If the maximum estimated error is larger than the chosen threshold, the machine performs a FP calculation. The threshold for the spilling factor was set to 0.02 following the literature [5]. For the Bayesian error, which exhibits a descriptor and material dependent non-zero value, the threshold is automatically determined on the fly. To this end, the machine stores the maximum value of the Bayesian errors for forces on the new structure that appeared just after the training step, where the force field was refined. Because this structure does not significantly differ from the structure sampled at the training step, the calculated Bayesian errors are nearly identical to the Bayesian errors on the already sampled structure. Hence, these calculated errors can be regarded as the lowest reachable Bayesian error, and their maximum value can provide a reasonable threshold for the Bayesian error to realize this reachable accuracy. In our algorithm, the criterion is updated by the average of the latest 10 stored maximum Bayesian errors when their relative standard deviation is smaller than 0.2.

*Sample selection*

As previously explained, MD simulations are performed, and whenever the machine decides that for a specific structure insufficient information is stored in the machine, FP calculations are performed for that structure. To reduce the computational demands, the machine is not retrained after each FP calculation, but instead retraining is done typically after $n$=5 FP calculations. This allows to block many of the computationally expensive steps in the training. When $n$ FP calculations have been done, local configurations are selected in a two-step procedure: (i) First, the machine examines the Bayesian error and spilling factor of each local configuration. If the

estimated errors are smaller than the threshold, the local configurations are disregarded. (ii) Next, the machine sparsifies the remaining local configurations by a CUR algorithm [3,6]. In our implementation, correlations between each local configuration and low rank singular values of the matrix *K* are examined by using leverage scorings. If the correlations are strong the corresponding local configuration is disregarded. Finally, the machine disregards those structure datasets that do not provide any local reference configurations to speed up the computations and to reduce the memory usage. The remaining structure datasets and local configurations are stored and used in subsequent learning updates.

## B. Models and parameters for training

Table B1 tabulates the conditions of the MD simulations used for the training of force fields. The simulations were executed on the 2×2×2 super cells shown in Fig. B1. For the training on each crystal, FP MD simulations in the *NPT* ensemble [7,8] were executed for the 2×2×2 supercell for 100 ps. Only for $MAPbI_3$, FP MD simulations in the *NVT* ensemble with the experimental volumes (see Refs. [10, 12] in the main text) were executed similarly to our previous FP MD studies (see Refs. [19-21] in the main text). Taking into account the available experimental data [9,10] (see also Refs.[10, 12, 29] in the main text), the temperature was set to the values tabulated in Table B1. For each material, the training was executed in the descending order of the table. Each training simulation started from an initial structure optimized by density-functional-theory (DFT) calculations [11,12]. As the initial structures for the optimizations of $MAPbI_3$ and $CsPbI_3$, experimental lattice structures (see Refs. [10, 12, 29] in the main text) were used while for other perovskites, the optimized $CsPbI_3$ structures were used. During the training of $MAPbI_3$, the mass of hydrogen was increased to 8.0 a.u. For the other perovskites, the original masses were adopted. This increased mass allows to set the time step to 3 fs for $MAPbI_3$. The time step for $CsPbCl_3$ was set to 3 fs, and that for other perovskites was set to 10 fs. All DFT calculations were performed using VASP (see Refs. [25, 26] in the main text). As electron exchange-correlation functional the SCAN functional (see Ref. [27] in the main text) was used, which was previously judged to provide the most accurate energetics on $MAPbI_3$ among several exchange-correlation functionals (see Ref. [20] in the main text). Relatively shallow pseudopotentials were used: for H $1s^1$, for C $2s^22p^2$, for N $2s^22p^3$, for Cl $3s^23p^5$, for Br $4s^24p^5$, for I $5s^25p^5$, for Cs $5s^25s^66s^1$, for Pb the $6s^26p^2$, and for Fr $6s^26s^67s^1$. The cutoff energy for the plane wave basis set was set to 350 eV for $MAPbI_3$, 287 eV for $CsPbI_3$ and $CsPbBr_3$, 341 eV for $CsPbCl_3$, and 280 eV for $FrPbI_3$ and $FrPbBr_3$. For the Brillouin zone integration, 4 Monkhorst-Pack **k**-points were used in all simulations. After training on the small super cells, simulations on larger super cells were performed without further refinement of the force fields.

**Table B1** Temperatures (K) of the MD simulations for the on-the-fly training. The pressure is set to 0.1 MPa in all simulations except for $MAPbI_3$, where the *NVT* ensemble was adopted.

| Material | Structure | Temperature | Material | Structure | Temperature |
|---|---|---|---|---|---|
| $MAPbI_3$ | Cubic | 450 | $CsPbCl_3$ | Cubic | 450 |
| | Tetragonal | 150 and 250 | | Tetragonal | 315 |
| | Orthorhombic | 150 | | Orthorhombic | 150 and 315 |
| $CsPbI_3$ | Cubic | 700 | $CsPbI_3$ | Cubic | 700 |
| | Tetragonal | 510 | | Tetragonal | 510 |
| | Orthorhombic | 150 and 325 | | Orthorhombic | 150 and 325 |
| $CsPbBr_3$ | Cubic | 500 | $FrPbBr_3$ | Cubic | 500 |
| | Tetragonal | 370 | | Tetragonal | 370 |
| | Orthorhombic | 150 and 370 | | Orthorhombic | 150 and 370 |

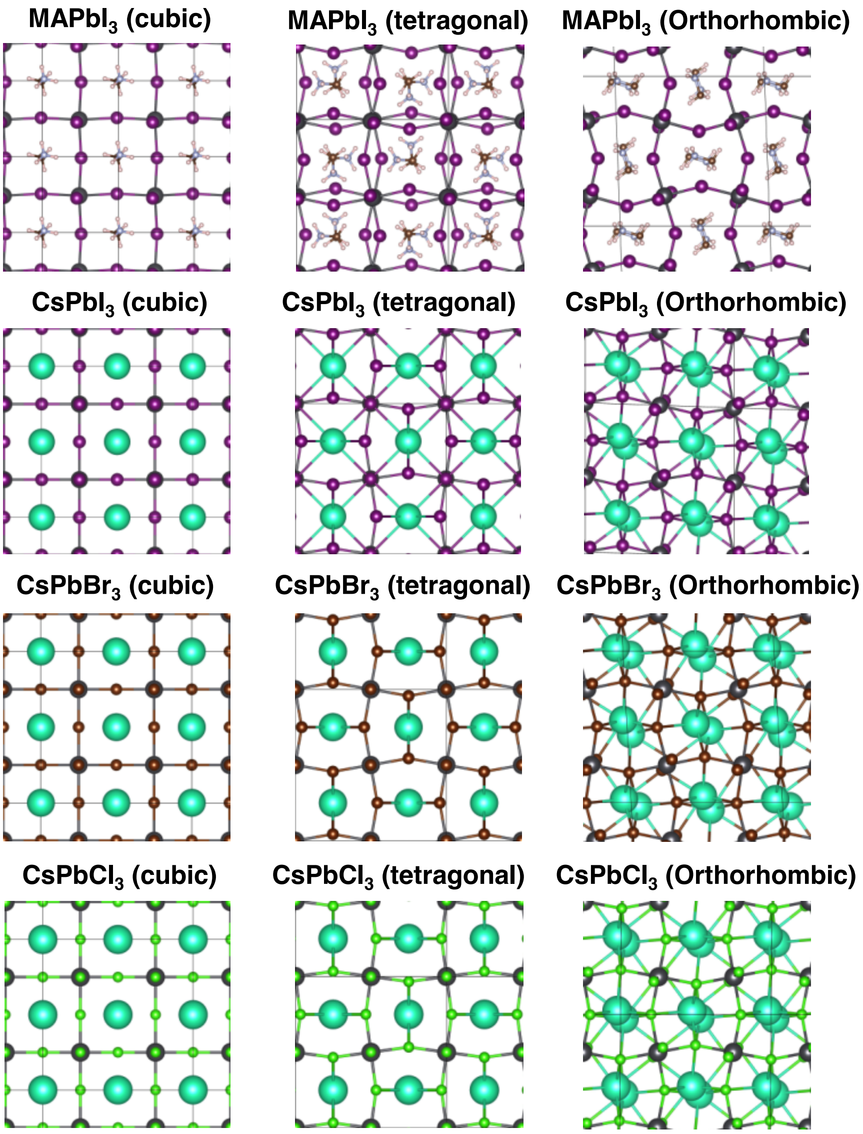


**Figure B1** 2×2×2 cells used for the training simulations. The structures for Fr perovskites are not shown because of strong similarity to Cs perovskites.

## C. Efficiency and accuracy

*Efficiency of training simulations*

Table C1 summarizes the fractions ($x_1$) of the MD steps, where FP calculations were bypassed, and the accelerations ($x_2=t_{FP}/t_{OTF}$) of the 100 ps MD simulations achieved by the on-the-fly scheme. Here, $t_{FP}$ denotes the time for a 100 ps FP MD simulation estimated from the timing per FP MD step, and $t_{OTF}$ denotes the actual elapsed time of the 100 ps on-the-fly MD simulation. The analysis indicates that, on average, 99 % of the FP calculations were bypassed, and the MD simulations were accelerated by almost a factor of 100 on average. The acceleration depends on the specific order of the training and the number of the total MD steps. For example, in $MAPbI_3$, the acceleration factor increases from the cubic to orthorhombic phase, i.e. when going down the table. This is because the training started from the cubic phase. At the beginning of the training on the orthorhombic phase, for example, the machine already possessed many reference datasets, and therefore, many FP calculations were bypassed. By the same reasoning, in a single MD run, the fraction of bypassed configurations gradually increases with the length of the simulation. Therefore, when the total number of the MD steps is set very large, as in the case of $MAPbI_3$ and $CsPbCl_3$, the bypassing fraction averaged over the MD simulation increases.

*Quality of the generated force fields*

Figures C1 and C2 show the root mean square errors in energy, forces and the stress tensor vs. the temperature. In this validation, 300 structures for each material were selected from a trajectory provided by a heating MD simulation on the 2×2×2 cells shown in Fig. B1. In these heating simulations, the generated force fields were used. On the collected configurations, DFT calculations were executed, and the calculated energies, forces and stress tensors were compared with the force fields. The root mean square errors averaged over all materials are 2.6 meV/atom for energies, 0.07 eV/Å for forces and 0.82 kbar for stress tensors. These are similar to the errors in the force fields for several other inorganic materials generated by conventional non on-the-fly schemes reported in past studies [2,13–16] (see also Ref. [1] in the main text).

Table C2 summarizes the number of structure datasets and the number of local configurations. The numbers of structure datasets $N_D$ are typically 500-900. All these numbers are surprisingly small compared with the typical numbers (2000-12000) used in past studies [2,13–16] (see also Ref. [1] in the main text). This is owed to the on-the-fly scheme that realizes efficient sampling on the target phenomena. Among the different perovskites, $CsPbI_3$ and $FrPbI_3$ need more training datasets than other perovskites because their training was carried out at higher temperature. $MAPbI_3$ also needs more datasets because the number of constituent elements of $MAPbI_3$ is larger than for other perovskites. Another impressive point is observed in the number of local configurations $N_B$ for each element type. Halide elements need more local reference configurations than other

elements. The trend is reasonably well explained by the fact that halides experience a variety of local chemical environments through ionic, hydrogen and van der Waals interactions with both $Pb^{2+}$ in the framework and a thermally fluctuating cation, $MA^+$, $Cs^+$ or $Fr^+$ (see Refs. [19, 21] in the main text, for example). Our on-the-fly scheme can automatically detect such element-dependent chemical environments and provides the necessary amount of local reference configurations for each element.

**Table C1** Fraction $x_1$ (%) of the number of MD steps, where FP calculations were bypassed, and the acceleration factor $x_2$ of a100 ps MD simulation achieved by the on-the-fly scheme. Values in the parentheses indicate the temperature.

| Material | Structure | $x_1$ | $x_2$ | Material | Structure | $x_1$ | $x_2$ |
|---|---|---|---|---|---|---|---|
| $MAPbI_3$ | Cubic (450) | 98.6 | 61 | $CsPbCl_3$ | Cubic (450) | 99.1 | 109 |
| | Tetragonal (250) | 99.5 | 123 | | Tetragonal (315) | 99.8 | 344 |
| | Tetragonal (150) | 99.5 | 112 | | Orthorhombic (315) | 99.7 | 247 |
| | Orthorhombic (150) | 99.8 | 196 | | Orthorhombic (150) | 99.8 | 311 |
| $CsPbI_3$ | Cubic (700) | 94.8 | 18 | $FrPbI_3$ | Cubic (700) | 95.3 | 21 |
| | Tetragonal (510) | 98.7 | 68 | | Tetragonal (510) | 98.8 | 75 |
| | Orthorhombic (325) | 99.1 | 96 | | Orthorhombic (325) | 99.0 | 87 |
| | Orthorhombic (150) | 99.2 | 84 | | Orthorhombic (150) | 99.4 | 144 |
| $CsPbBr_3$ | Cubic (500) | 97.7 | 42 | $FrPbBr_3$ | Cubic (500) | 97.7 | 41 |
| | Tetragonal (370) | 98.8 | 73 | | Tetragonal (370) | 99.2 | 114 |
| | Orthorhombic (370) | 98.5 | 59 | | Orthorhombic (370) | 98.8 | 72 |
| | Orthorhombic (150) | 99.3 | 118 | | Orthorhombic (150) | 99.3 | 123 |

**Table C2** Number of structure datasets, $N_D$, providing the training data and local reference configurations, and the number of local reference configurations, $N_B$, for each element type.

| Material | $N_D$ | $N_B$ | Material | $N_D$ | $N_B$ |
|---|---|---|---|---|---|
| $MAPbI_3$ | 724 | 219 (Pb) | $CsPbCl_3$ | 547 | 135 (Pb) |
| | | 1209 (I) | | | 740 (Cl) |
| | | 87 (C) | | | 116 (Cs) |
| | | 97 (N) | | | |
| | | 743 (H) | | | |
| $CsPbI_3$ | 845 | 135 (Pb) | $FrPbI_3$ | 755 | 137 (Pb) |
| | | 1331 (I) | | | 1180 (I) |
| | | 235 (Cs) | | | 221 (Fr) |
| $CsPbBr_3$ | 572 | 187 (Pb) | $FrPbBr_3$ | 503 | 146 (Pb) |
| | | 1068 (Br) | | | 822 (Br) |
| | | 224 (Cs) | | | 167 (Fr) |

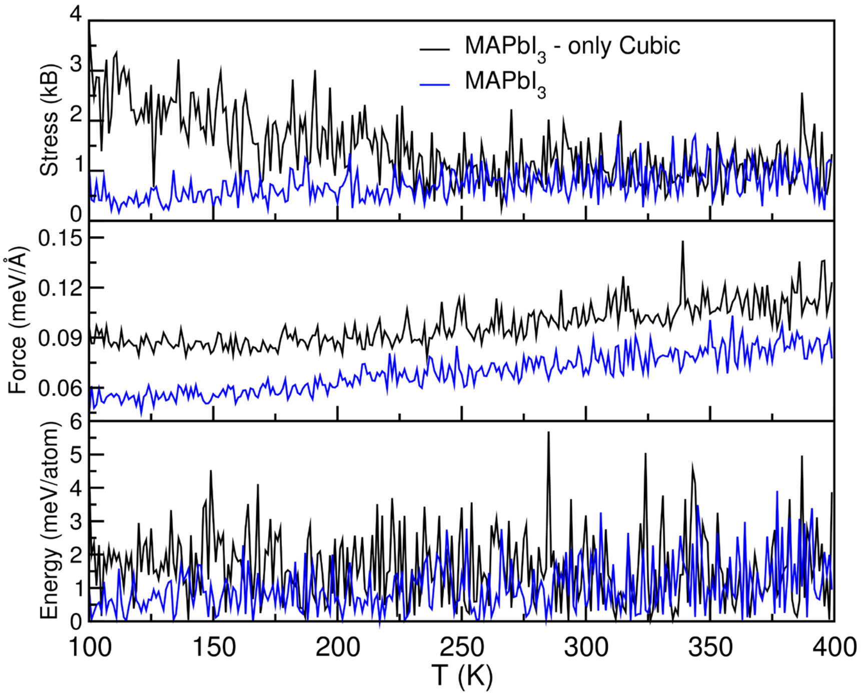


**Figure C1** Root mean square errors in energy, forces and stress tensor of the MLFF trained on all three phases of $MAPbI_3$ (blue line) and trained only on the cubic $MAPbI_3$ (black line). The former MLFF is used in this work.

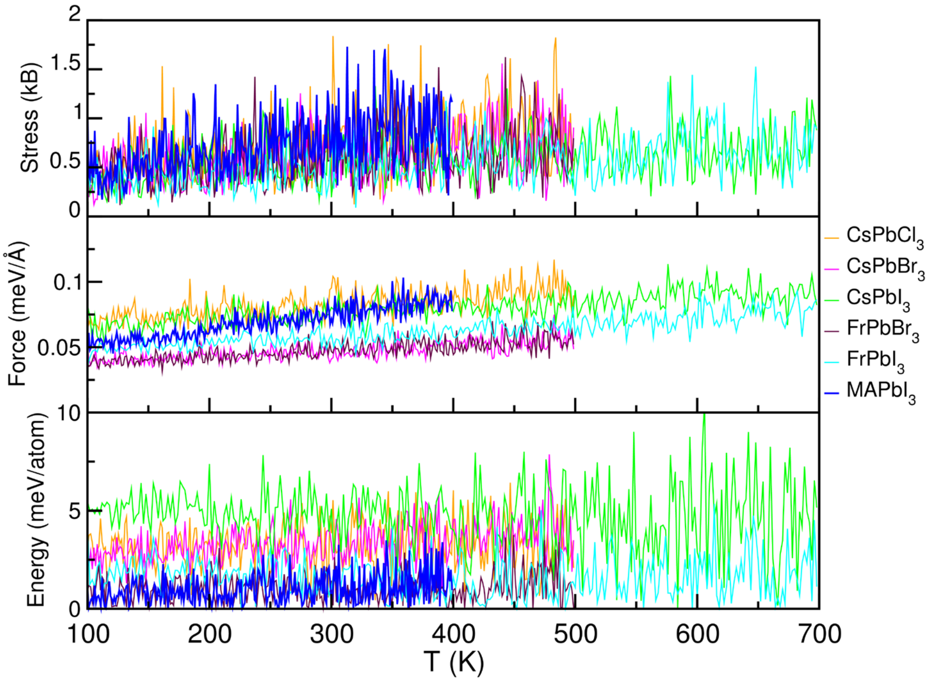


**Figure C2** Root mean square errors in energy, forces and stress tensor of MLFF trained on all three phases of $ABX_3$ (A=Cs or Fr, B=Pb, and X=I, Br or Cl).

*Efficiency of the force-field calculations*

The measured elapsed time per MD step for $MAPbI_3$ is shown in Table C3. In the test calculations, we used 16 and 48 Intel® XEON® E5-2650 (v2) 2.60 GHz cores for the 2×2×2 and 4×4×4 cells, respectively, in both MLFF and DFT calculations. The DFT calculations on the 2×2×2 cell were executed using the parameters explained in Section B. For the DFT calculation on the 4×4×4 cell, a single **k**-point (Γ-point) was used. Other parameters are the same as those for the 2×2×2 cell. The force field is approximately 300 and 1000 times faster than DFT for the 2×2×2 and 4×4×4 cells, respectively.

**Table C3** Elapsed time (s) per MD step on $MAPbI_3$ by the MLFF and DFT.

| System | MLFF | DFT |
|---|---|---|
| 2×2×2 (96 atoms) | 0.49 | 146.1 |
| 4×4×4 (768 atoms) | 1.32 | 1106.0 |

## D. Simulations of phase transitions using force fields

### D.1 Simulations on $MAPbI_3$

The lattice constants of $MAPbI_3$ shown in Fig. 2 were obtained using 4×4×4 unit cells involving two steps: (i) determination of the phase transition temperatures by heating and cooling, and (ii) evaluation of the equilibrium lattice constants for the stable phase at the considered temperatures by fitting Gaussian functions to the distribution function of the lattice constants. The precise phase transition temperatures were determined either by extensive constant-temperature MD simulations or by using free-energy analysis relying on the umbrella-integration method (see Ref. [28] in the main text). *NPT* simulations [7,8] were carried out for 0.2-1.2 ns for the relevant phase. In all simulations, the mass of hydrogen was increased to 4.0 a.u. and the time step was set to 2.0 fs. Further details of the simulations are explained in the following subsections.

*Rough estimations of transition temperatures by heating, cooling and constant temperature MD simulations*

Heating and cooling MD simulations were carried out on the 4×4×4 cell. As shown in Fig. 3(a) in the main text for the heating and Fig. D1 for the cooling, the simulations with a heating (or cooling) rate of 0.5 K/ps exhibit reversible transitions between the tetragonal and cubic phase at around 370 K. The heating simulation also shows the orthorhombic to tetragonal phase transition in the temperature range between 200 and 270 K. However, the reverse phase transition is not observed in the cooling simulation because of the slow kinetics of this ordering transition at low temperature. In order to narrow the uncertainty of this transition temperature, further simulations were carried out. The heating simulations with several heating rates shown in Fig. D2 indicate that the transition range gradually decreases to 200-250 K with decreasing heating rate. However, the reverse phase transition was not observed even when the cooling rate was decreased to 0.25 K/ps (not shown in the figure). An MD simulation for 1.2 ns at 200 K, which started from the 4×4×4 orthorhombic cell, did not show the orthorhombic to tetragonal phase transition. In contrast, as indicated in Fig. D3, a simulation at 220 K shows the orthorhombic to tetragonal phase transition, where the transition of the $PbI_6$ frame occurs *after* the reorganization of the molecules similarly to the heating simulation shown in Fig. 3(b). These results allow to estimate that the transition temperature is approximately 200-220 K.

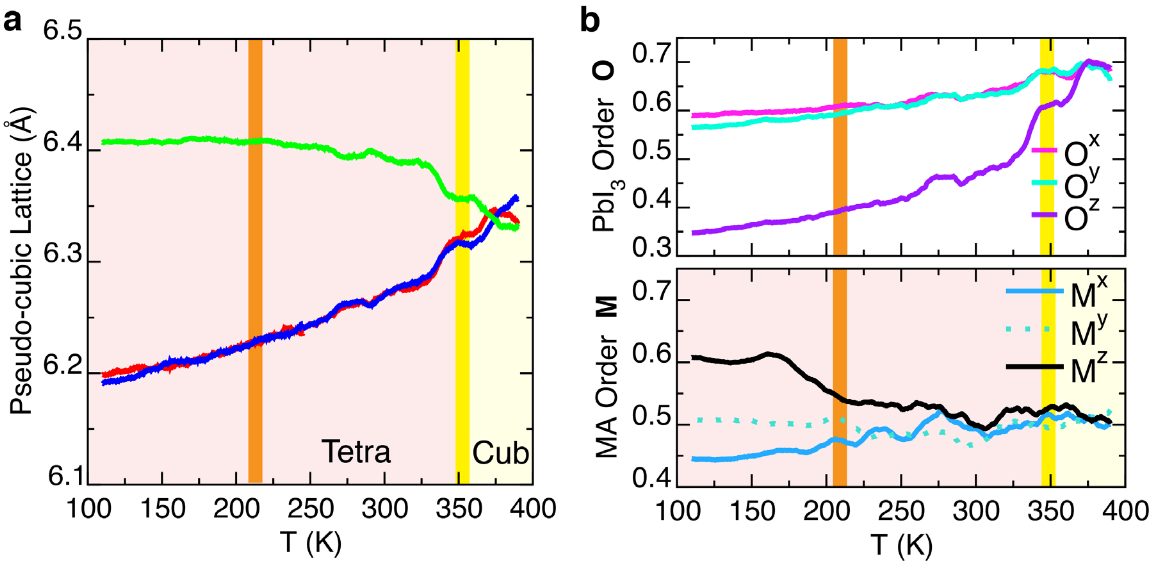


**Figure D1** Cooling simulation for a 4×4×4 cell of $MAPbI_3$ at a cooling rate of 0.5 K/ps. Pseudo-cubic lattice constants (**a**) and frame and molecular order parameters (**b**).

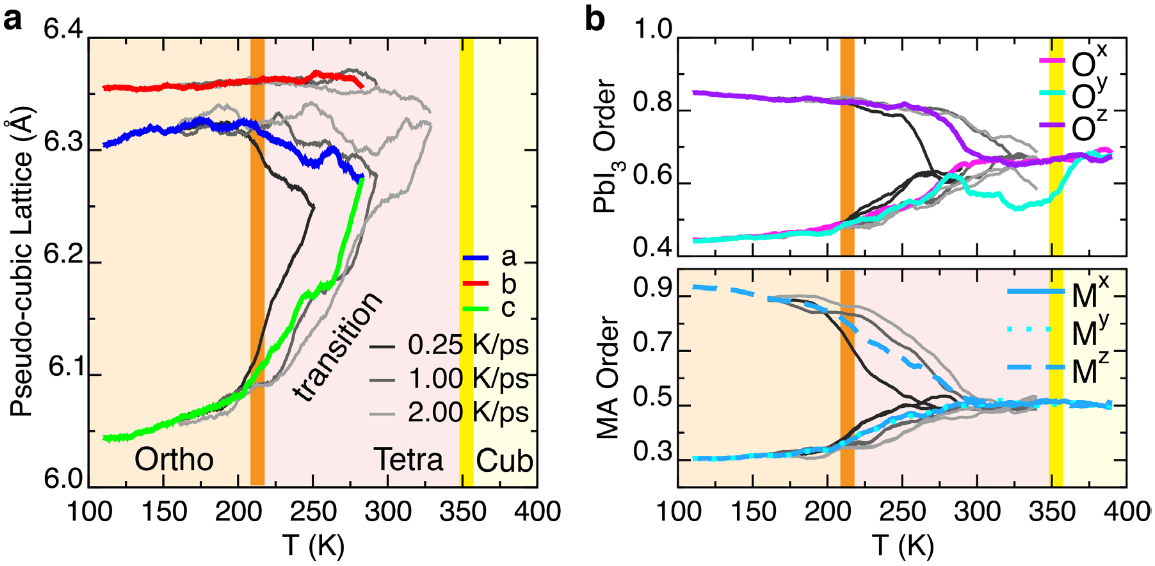


**Figure D2** Heating simulations for a 4×4×4 cell of $MAPbI_3$ at heating rates of 0.25, 0.50, 1.00 and 2.00 K/ps. Pseudo-cubic lattice constants (**a**) and (**b**) frame and molecular order parameters.

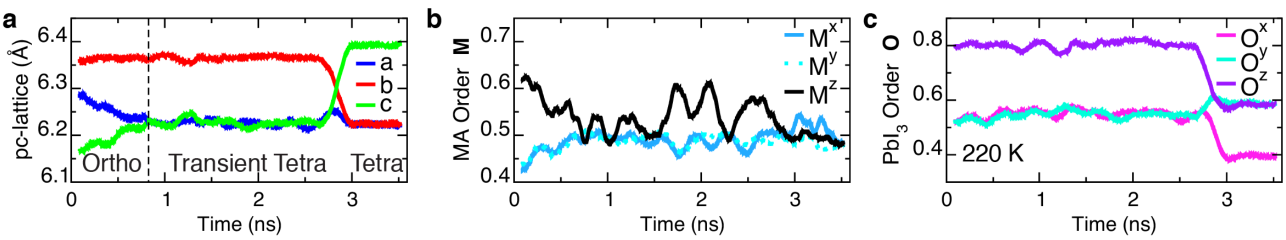


**Figure D3** Constant temperature MD simulation at 220 K for a 4×4×4 cell of $MAPbI_3$. Lattice constants (**a**), molecular order parameter (**b**) and frame order parameter (**c**).

*Free energy analysis and orthorhombic to tetragonal phase transition temperature*

For a more precise determination of the orthorhombic to tetragonal transition temperature, we carried out a free energy analysis for a 4×2×2 cell using the umbrella integration scheme. In this scheme, bias spring potentials are introduced in order to constrain the collective variables $\xi_k$ of the system to certain window values $\xi_{wk}$. Using the constraints, samplings of rare configurations become feasible. If the spring constant is much larger than the curvatures of the unbiased potential energy surface, the probability distribution along the collective variables obeys a Gaussian distribution. This condition allows to calculate the derivatives of the potential of the mean force with respect to the collective variables as,

$$\frac{\partial W}{\partial \xi_k} = k_B T \frac{\xi_k - \bar{\xi}_{wk}}{\sigma_{wk}^2} - k_0(\xi_k - \xi_{wk}). \qquad \text{(D1)}$$

Here, $k_B$ is the Boltzmann constant, $\bar{\xi}_{wk}$ and $\sigma_{wk}^2$ are the mean value and variance of the collective variable $\xi_k$ obtained by the MD simulation with the bias potential, and $k_0$ is a force constant. By integrating the calculated derivatives along the collective variables, the potential of the mean force (free energy) is calculated. In this study, we adopted a simple numerical integration method using the derivatives, $-k_0(\bar{\xi}_{wk} - \xi_{wk})$, at $\xi_k = \bar{\xi}_{wk}$. As the collective variables, the dihedral angles between two adjacent $PbI_6$ octahedra along the $z$-axis were used. The number of the windows was set to 14 after checking the convergence of the calculated free energy curves. The force constant $k_0$ was set to 50 eV/rad$^2$, which is sufficiently larger than the curvature ($\kappa_{TS} \approx 2$ eV/rad$^2$ per cell) of the calculated free energy curves at the transient point. At each window, a 0.3 ns MD simulation using an *NPT*-ensemble was executed to obtain $\bar{\xi}_{wk}$ and $\sigma^2_{wk}$. Error propagation analyses [17] indicate

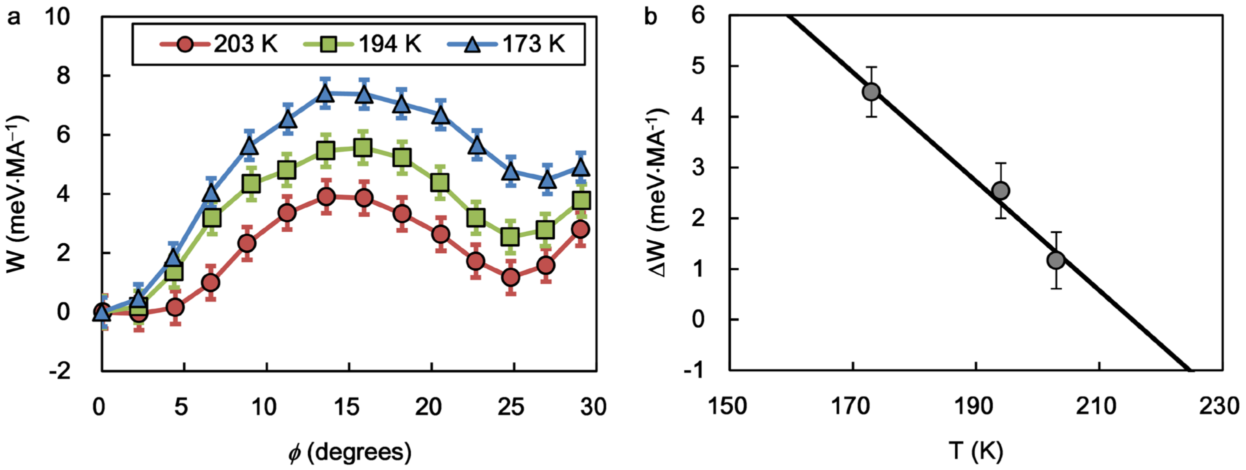


**Figure D4** (**a**) Potential of the mean force $W$ vs. dihedral angle $\phi$ between two adjacent $PtI_6$ octahedra along $z$-axis. The orthorhombic and tetragonal phases are located at the two minima at $\phi$ = 0 and 25 °, respectively. (**b**) Free energy difference $\Delta W$ between the two minima in the free energy curve vs. the temperature. A negative sign of $\Delta W$ indicates that the tetragonal phase is more stable than the orthorhombic phase.

error bars of ±10 meV per cell for the free energy curves. Figure D4(a) shows the free energy curves at 173, 194 and 203 K as a function of the dihedral angle $\phi$. The free energy of the tetragonal phase located at $\phi$=25° relative to that of the orthorhombic phase located at $\phi$=0° decreases with increasing temperature. The linear fitting of the free energy difference $\Delta W$ between the tetragonal and orthorhombic phase vs. the temperature shown in Fig. D4(b) provides a transition temperature of 215±10 K and a change of the entropy at the phase transition of 1.3±0.6 $k_B$.

*Equilibrium lattice constants and tetragonal to cubic phase transition temperature*

After the simulations explained in the previous two subsections, MD simulations on the 4×4×4 cell at various temperatures, ranging from 100 to 400 K, were carried out to determine the equilibrium lattice parameters. The MD-simulation time was set to 0.2 ns except for 200 K. At 200 K, the simulation time was increased to 1.2 ns because the structure only very slowly converged at this temperature near the phase transition point.

Close to the tetragonal to cubic transition temperature the unit cell undergoes frequent fluctuations between these two phases. Therefore, it is very difficult to uniquely determine at any point in time, whether the structure is in the tetragonal, cubic, or in a transition state. We therefore constructed a combined distribution function $\rho(x)$ of the pseudo-cubic lattice parameters $a$, $b$ and $c$ from the MD trajectory and fitted Gaussian functions to it as follows,

$$\rho(x) = \sum_{i=1}^{n} \frac{1}{\sqrt{2\pi\sigma_i^2}} \exp\left(-\frac{(x-\mu_i)}{2\sigma_i^2}\right), \quad \text{(D2)}$$

where $\mu_i$ and $\sigma_i$ are the equilibrium lattice parameters and their variances. The optimization of $\mu_i$ and $\sigma_i$ was carried out by the following procedure. First, three Gaussian functions are fitted to $\rho(x)$. When the differences between the optimized lattice parameters are larger than $\sqrt{}(\sigma_1^2+\sigma_2^2+\sigma_3^2)/3$, the distribution is judged to be orthorhombic. If not, two Gaussians are fitted, and the difference in the optimized lattice parameters is examined. If the difference is larger than $\sqrt{}(\sigma_1^2+\sigma_2^2)/2$, the distribution is judged to be tetragonal. Otherwise the distribution is judged to be cubic, and a single Gaussian is fitted. Figure 1(a) of the main text shows the result of this procedure. To illustrate the procedure, we show the calculated distribution functions at 100, 208, 342 and 367 K in Fig. D5.

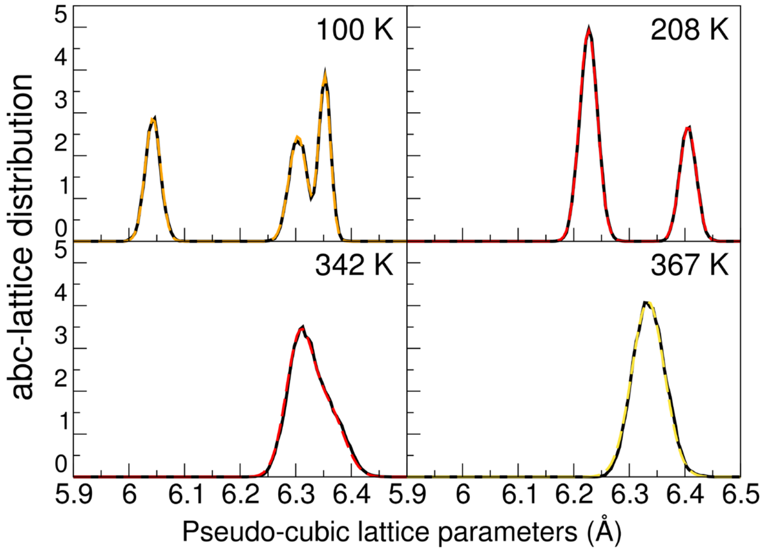


**Figure D5** Combined distribution function $\rho(x)$ of the psuedo-cubic lattice parameters $a$, $b$ and $c$ at 100, 208, 342 and 367 K. Solid lines show the distributions constructed from the MD trajectories, and dashed lines are the fitted Gaussian distributions. The fitting procedure identifies the orthorhombic structure at 100 K, tetragonal structures at 208 and 342 K, and the cubic structure at 367 K.

### D.2 Simulations on inorganic perovskites

Since the other perovskites exhibit reversible phase transitions, the phase transition temperatures were simply calculated as the average of the observed transition temperatures for heating and cooling in *NPT* simulations. The lattice constants provided by these two simulations are plotted in Fig. 3(a) showing negligible hysteresis. In the MD simulations, the mass of Cl was increased to 79.904 a.u., and the time step was set to 10 fs. All calculations were done using 6×6×6 unit cells. The larger cells (compared to $MAPbI_3$) were feasible, because the time step for the simulation can be chosen much larger for inorganic perovskites, and because the dynamics is generally faster in inorganic perovskites, as there is no hindered slow reorientation of the MA molecules. Figures D6 and D7 show the simulated pseudo-cubic lattice parameters vs. the temperature obtained during the heating and cooling simulations. The determined phase transition temperatures are shown in the same figure. The orthorhombic to tetragonal transition temperature was determined as the point, where the pseudo-cubic lattice constants merge (or split). The tetragonal to cubic phase transition temperature was determined as the point, where the pseudo-cubic lattice parameters merge (or split) and the frame order parameters merge (or split). An average value between the heating and cooling runs was used as the phase transition temperature, and its error bar was set to the spread between these two values.

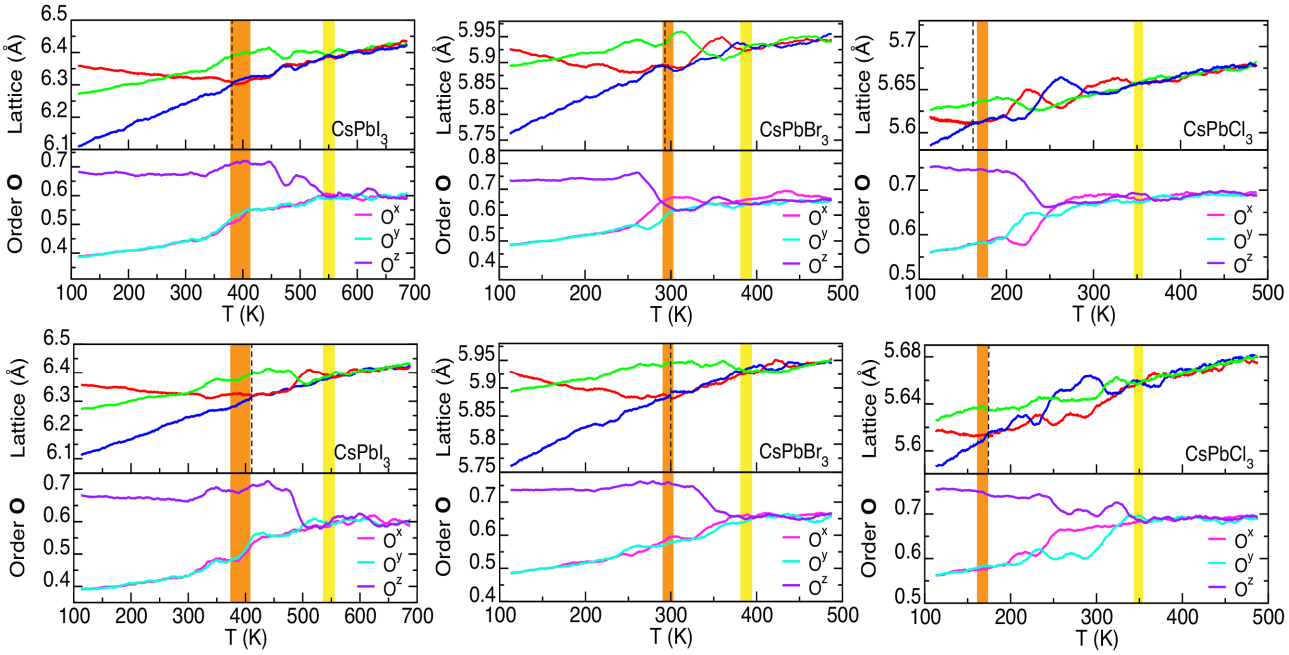


**Figure D6** Pseudo-lattice constants and frame order provided by the cooling (upper panels) and heating (lower panels) simulations on the 6×6×6 super cells of $CsPbI_3$, $CsPbBr_3$ and $CsPbCl_3$. Orange and yellow color bars are the orthorhombic to tetragonal and tetragonal to cubic transition temperatures, respectively.

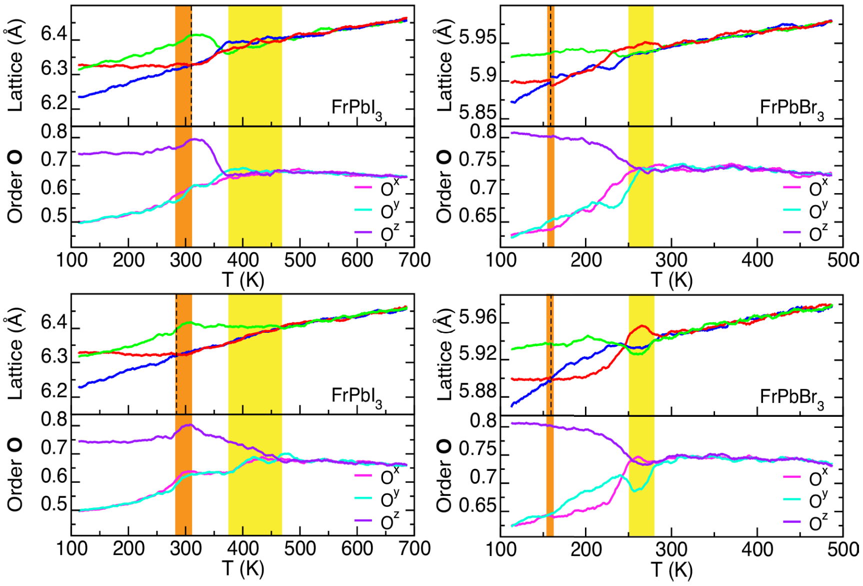


**Figure D7** Pseudo-lattice constants and frame order provided by the cooling (upper panels) and heating (lower panels) simulations on the 6×6×6 super cells of $FrPbI_3$ and $FrPbBr_3$. Orange and yellow color bars are the orthorhombic to tetragonal and tetragonal to cubic transition temperatures, respectively.

## E. Order parameters

*Frame order parameter*

A major difference in the frame pattern is in the dihedral angles of adjacent $PbI_6$ octahedra. For example, as shown in Fig. 2(d) or Fig. 3(e), the dihedral angles of adjacent octahedra along the $z$-axis are nearly zero in the orthorhombic phase, while they are 20-25° in the tetragonal phase. This difference can be described by the frame order parameter. For the formulation of the frame order parameter, we introduce an integer cubic grid $\mathbf{q}=(i, j, k)$ with dimensions of $N_{\mathrm{unit}} = N_x \times N_y \times N_z$, which specifies the position of each $PbI_6$ octahedron. For each octahedron, we define three unit vectors $\hat{\mathbf{I}}_{\mathbf{q}}^{\beta}$ ($\beta$=$x$, $y$ or $z$), which measure the orientation of the I-I vectors in the octahedron as shown in Fig. 3(b). The frame order parameter, $\mathbf{O} = (O^x, O^y, O^z)$, is defined as follows,

$$O^{\alpha} = \prod_{\mathbf{q}} \prod_{\beta \neq \alpha} \left( \hat{\mathbf{I}}_{\mathbf{q}}^{\beta} \cdot \hat{\mathbf{I}}_{\mathbf{q}+\mathbf{e}^{\alpha}}^{\beta} \right)^{4/N_{\mathrm{unit}}}, \tag{E1}$$

where $\mathbf{e}^{\alpha}$ is a displacement unit vector to a neighboring site in the direction $\alpha$.

*Molecular order parameter*

In a similar manner, the molecular order parameter $\mathbf{M} = (M^x, M^y, M^z)$ is defined as,

$$M^{\alpha} = \frac{1}{\pi N_{\mathrm{unit}}} \sum_{\mathbf{q}} \arccos\left( \hat{\mathbf{p}}_{\mathbf{q}} \cdot \hat{\mathbf{p}}_{\mathbf{q}+\mathbf{e}^{\alpha}} \right), \tag{E2}$$

where $\hat{\mathbf{p}}_{\mathbf{q}}$ is the C-N unit vector of an MA molecule on the grid point $\mathbf{q}$. This order parameter measures the correlation between orientations of two adjacent MA molecules. In the orthorhombic phase, for example, the C-N vector of one MA molecule is nearly antiparallel to that of an adjacent MA molecule along the $z$-axis as shown in Fig. 2(d). Thus, the order parameter $M^z$ approaches unity. On the other hand, the angular correlations in the remaining two directions are weak, and therefore, $M^x$ and $M^y$ become close to 0.5. In the tetragonal phase, the adjacent molecules in the $x$- and $y$-directions are nearly orthonormal (90°), and therefore, the order parameter is close to 0.5. In the $c$-direction the angles are slightly larger than 90°. In the cubic phase, all angular correlations are weak, and therefore, the order parameters in all directions approach to 0.5.

## F. Reorientation time of MA molecules

The reorientation time of MA molecules in $MAPbI_3$ was determined by fitting a linear combination of two exponential functions, $A \exp(-t/\tau_1) + (1-A) \exp(-t/\tau_2)$, to the autocorrelation function of the MA molecular orientations obtained by the MD simulation at constant temperature. Here, the autocorrelation function is calculated as described in Ref. [19] in the main text. Figure F1 shows the autocorrelation functions, and the optimized parameters are tabulated in Table F1. The fitting provides two decay times: the longer decay time $\tau_1$ for the molecular reorientations and the shorter decay time $\tau_2$ for the thermal fluctuations.

**Table F1** Parameters in the exponential functions, $A \exp(-t/\tau_1) + (1-A) \exp(-t/\tau_2)$, optimized to the autocorrelation functions of the MA molecular orientations in $MAPbI_3$. $\tau_1$ represents the MA molecular reorientation time.

| $T$ (K) | $A$ | $\tau_1$ (ps) | $\tau_2$ (ps) | $T$ (K) | $A$ | $\tau_1$ (ps) | $\tau_2$ (ps) |
|---|---|---|---|---|---|---|---|
| 150 | 0.96 | 19405.2 | 0.3 | 250 | 0.88 | 36.3 | 0.5 |
| 175 | 0.92 | 711.1 | 0.4 | 300 | 0.87 | 11.5 | 0.5 |
| 200 | 0.90 | 195.5 | 0.9 | 350 | 0.83 | 6.4 | 0.6 |
| 208 | 0.90 | 103.1 | 0.4 | 400 | 0.87 | 3.5 | 0.5 |

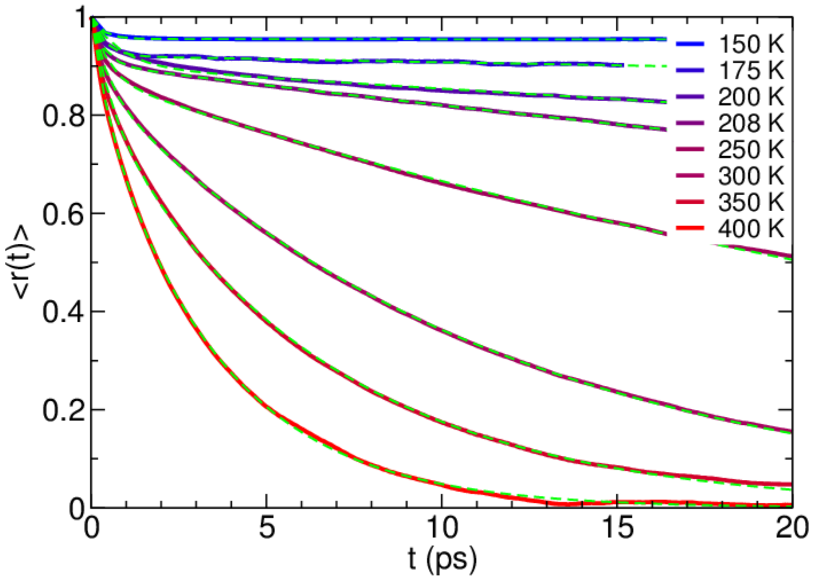


**Figure F1** Autocorrelation functions of the MA molecular orientations. Dashed lines show the exponential functions fitted to the autocorrelation functions.

## G. Ionic radii and Goldschmidt tolerance factors

Table G1 summarizes the ionic radii and Goldschmidt tolerance factors used to obtain the data in Fig. 3(d). The conventional empirically-determined ionic radii were used except for Fr and MA [18]. In the case of Fr, we determined the ionic radius as $r_{Cs}+\sqrt{3}\Delta L/2$, where $r_{Cs}$ is the ionic radius of Cs, and $\Delta L$ is the average of the differences in the theoretically obtained lattice constants of FrX and CsX (X=I, Br or Cl) in the CsCl crystal structure. The obtained lattice constants are tabulated in Table G2. These lattice constants were obtained by DFT calculations using the SCAN functional on the primitive cells of the ionic crystals. A 6×6×6 **k**-point mesh was used, and the cutoff energy was set as 287 eV for CsI, CsBr, FrI and FrBr, and 341 eV for CsCl and FrCl. For the ionic radius of MA, we adopted the radius determined in Ref. [19], where a rigid sphere model with free rotation around its center of mass was applied.

**Table G1** Ionic radii $r_s$ (Å), where $s$ denotes the ionic species, and Goldschmidt tolerance factors $t$ of perovskites $ABX_3$ (A= MA, Cs or Fr, and X=Cl, Br or I).

| Material | $r_A$ | $r_{Pb}$ | $r_X$ | $t$ |
|---|---|---|---|---|
| $MAPbI_3$ | 1.74 | 1.19 | 2.20 | 0.819 |
| $CsPbI_3$ | 1.67 | 1.19 | 2.20 | 0.807 |
| $CsPbBr_3$ | 1.67 | 1.19 | 1.96 | 0.815 |
| $CsPbCl_3$ | 1.67 | 1.19 | 1.81 | 0.820 |
| $FrPbI_3$ | 1.73 | 1.19 | 2.20 | 0.814 |
| $FrPbBr_3$ | 1.73 | 1.19 | 1.96 | 0.822 |

**Table G2** Lattice constants $L$ (Å) of CsX and FrX crystals in the CsCl structure obtained by DFT calculations using the SCAN functional.

| Material | $L$ | Material | $L$ |
|---|---|---|---|
| CsI | 4.645 | FrI | 4.730 |
| CsBr | 4.295 | FrBr | 4.402 |
| CsCl | 4.101 | FrCl | 4.177 |

## H. Supplementary Movies

The lattice parameters and order parameters presented in this work provide an accurate description of the transition during the MLFF MD run. Still, a movie can be helpful to gain a more intuitive grasp. We have therefore made four illustrative movies of $MAPbI_3$.

- **SMovie 1:** Movie showing the structural deformation of the 4×4×4 MAPbI3 cell during the heating simulation from 100 to 400 K as shown in Figs. 3(a) and (b) of the main text. The orthorhombic phase turns into the tetragonal phase and consecutively to the cubic phase.
- **SMovie 2:** Movie showing the structural deformation of the 4×4×4 MAPbI3 cell during a cooling simulation from 400 to 100 K. The structure transforms from the cubic phase into the tetragonal phase and freezes in.
- **SMovie 3:** Movie showing the structural relaxation of an 8×2×2 Orthorhombic-Tetragonal interface structure at constant temperature of ~175 K. At the end of the movie the interface is annihilated and a continuous orthorhombic phase remains.
- **SMovie 4:** Movie showing the structural relaxation of an 8×2×2 Orthorhombic-Tetragonal interface structure at constant temperature of ~225 K. At the end of the movie the interface is annihilated and a continuous tetragonal phase remains.

The movies can be downloaded from:
http://www.dynamicsolids.net/sm/2019-mlff-perovskites

## References in Supplementary Materials


[1] W. J. Szlachta, A. P. Bartók, and G. Csányi, Phys. Rev. B **90**, 104108 (2014).

[2] V. L. Deringer, N. Bernstein, A. P. Bartók, M. J. Cliffe, R. N. Kerber, L. E. Marbella, C. P. Grey, S. R. Elliott, and G. Csányi, J. Phys. Chem. Lett. **9**, 2879 (2018).

[3] V. L. Deringer and G. Csányi, Phys. Rev. B **95**, 94203 (2017).

[4] A. P. Bartók, S. De, C. Poelking, N. Bernstein, J. R. Kermode, G. Csányi, and M. Ceriotti, Sci. Adv. **3**, e1701816 (2017).

[5] K. Miwa and H. Ohno, Phys. Rev. B **94**, 184109 (2016).

[6] M. W. Mahoney and P. Drineas, Proc. Natl. Acad. Sci. U. S. A. **106**, 697 (2009).

[7] M. Parrinello and A. Rahman, Phys. Rev. Lett. **45**, 1196 (1980).

[8] M. Parrinello and A. Rahman, J. Appl. Phys. **52**, 7182 (1981).

[9] C. C. Stoumpos, C. D. Malliakas, J. A. Peters, Z. Liu, M. Sebastian, J. Im, T. C. Chasapis, A. C. Wibowo, D. Y. Chung, A. J. Freeman, B. W. Wessels, and M. G. Kanatzidis, Cryst. Growth Des. **13**, 2722 (2013).

[10] Y. Fujii, S. Hoshino, Y. Yamada, and G. Shirane, Phys. Rev. B **9**, 4549 (1974).

[11] P. Hoenberg and W. Kohn, Phys. Rev. **136**, B864 (1964).

[12] W. Kohn and L. J. Sham, Phys. Rev. **140**, A1133 (1965).

[13] T. Morawietz, A. Singraber, C. Dellago, and J. Behler, Proc. Natl. Acad. Sci. **113**, 8368 LP (2016).

[14] N. Artrith and A. Urban, Comput. Mater. Sci. **114**, 135 (2016).

[15] S. Chiriki, S. Jindal, and S. S. Bulusu, J. Chem. Phys. **146**, 84314 (2017).

[16] S. Faraji, S. A. Ghasemi, S. Rostami, R. Rasoulkhani, B. Schaefer, S. Goedecker, and M. Amsler, Phys. Rev. B **95**, 104105 (2017).

[17] J. Kästner and W. Thiel, J. Chem. Phys. **124**, 234106 (2006).

[18] V. M. Goldschmidt, Berichte Der Dtsch. Chem. Gesellschaft (A B Ser. **60**, 1263 (1927).

[19] J. Navas, A. Sánchez-Coronilla, J. J. Gallardo, E. I. Martín, N. C. Hernández, R. Alcántara, C. Fernández-Lorenzo, and J. Martín-Calleja, Phys. Chem. Chem. Phys. **17**, 23886 (2015).
